# Supplementary material for: State Predictive Information Bottleneck
Source: arXiv:2011.10127 ancillary file (2021-02-12)
Supplement: Supplementary file 1 [file SM.pdf]

# Supplementary Material: State Predictive Information Bottleneck

**Wang and Tiwary**

## I. DETERMINING $\beta$ VIA THE TRADE-OFF BETWEEN RATE AND DISTORTION

As discussed in the main text, the objective function of the information bottleneck (IB) can be written into two parts (the entropy of the targets has been ignored):

$$\begin{aligned}\mathcal{L} \approx & -\underbrace{\frac{1}{N}\sum_{n=1}^{N}\int d\boldsymbol{z}\Big[-p(\boldsymbol{z}|\boldsymbol{X}^n)\log q(\boldsymbol{y}^n|\boldsymbol{z})\Big]}_{distortion} \\ & -\beta\ \underbrace{\frac{1}{N}\sum_{n=1}^{N}\int d\boldsymbol{z}\Big[p(\boldsymbol{z}|\boldsymbol{X}^n)\log\frac{p(\boldsymbol{z}|\boldsymbol{X}^n)}{r(\boldsymbol{z})}\Big]}_{rate}\end{aligned} \tag{1}$$

Based on rate-distortion theory,[1,2] the first term in Eq. 1 can be interpreted as the distortion, which measures the ability of our representation to predict the desired target, while the second term can be interpreted as the rate, which measures the number of bits per data sample to be transmitted. Reducing the rate will limit the ability of $\boldsymbol{z}$ to predict the target, increasing the distortion. Therefore, maximizing this objective function results in a competition between the rate and the distortion. Such a trade-off can be controlled by the hyper-parameter $\beta$. In principle, an ideal $\beta$ will utilize every byte transmitted with maximum efficiency to predict the target. In this work, we chose the turning point of the Rate-Distortion plot as the optimum $\beta$ in order to obtain a maximally informative representation. However, we also found that as long as $\beta$ is not too large, its value will not have a big impact on our results.

## II. ESTIMATING THE TIMESCALE OF THE UNDERLYING DYNAMICS

As we did in the main text, we can derive a spectral decomposition for the propagator $\mathcal{P}(\tau)$ by assuming $\boldsymbol{X}_t$ is reversible:[3]

$$\rho_\tau = v_1 + \sum_{i=2}^{\infty} a_i(\rho_0)\lambda_i(\tau)v_i \tag{2}$$

where $\{v_i\}$ are the propagator's eigenfunctions and $\lambda_i = \exp(-k_i\tau)$ are the eigenvalues which decay exponentially in time with rates $k_i$. Then $t_i = 1/k_i$ can represent the corresponding timescale of the underlying dynamics. One way to estimate the eigenfunctions and the

eigenvalues in Eq. 2 is by constructing a Markov state model (MSM).[4,5] Given the state label function $\boldsymbol{h}(\boldsymbol{X})$, we can easily obtain the transition probability matrix $\boldsymbol{\mathcal{T}}(\tau) = \{\mathcal{T}_{ij}(\tau)\}$ within a given lag time $\tau$ through data samples:

$$\mathcal{T}_{ij}(\tau) = \frac{\sum_{n=1}^{M} h_i(\boldsymbol{X}^{n+k}) h_j(\boldsymbol{X}^n)}{\sum_{n=1}^{M} h_j(\boldsymbol{X}^n)} \tag{3}$$

where the time interval between $\boldsymbol{X}^n$ and $\boldsymbol{X}^{n+k}$ is the lag time $\tau$, and $i, j$ are any two states. The eigenvalues $\{\hat{\lambda}_i\}$ of $\boldsymbol{\mathcal{T}}(\tau)$ then can be used to estimate the different relaxation timescales of the molecular system:

$$\hat{t}_i(\tau) = -\frac{\tau}{\ln |\lambda_i(\tau)|} \tag{4}$$

Here, $\hat{t}_i(\tau)$ is called the implied timescale corresponding to the $i^{th}$ eigenvalue $\{\hat{\lambda}_i\}$. Note that in principle we will always have $\hat{\lambda}_1 = 1$ and $\hat{t}_1 = \infty$ as the corresponding eigenfunction represents the stationary distribution.

## III. GENERATING THE INITIAL STATE LABELS THROUGH THE DISCRETIZATION

As shown in the main text, the State Predictive Information Bottleneck (SPIB) is very robust to the initial state labels. Basically, as long as the state labels can somewhat distinguish between different metastable states, they can be used to initialize our algorithm. For alanine dipeptide, we also tried another two sets of initial state labels generated by discretizing the input data along $\psi$ and $\theta$ respectively. We found SPIB was still able to work very well on the initial state labels generated by $\psi$ (as shown in Supplementary Fig. 7), but failed on those generated by $\theta$. Supplementary Fig. 9 explained the reason–though $\theta$ is important for identifying the transition states (as illustrated in the main text), it is really a bad order parameter in the sense that it alone cannot distinguish the basins at all. Thus, as we expected, the state labels generated from $\theta$ were purely misleading and resulted in the failure of our algorithm.

## IV. DOUBLE-WELL ANALYTICAL POTENTIAL

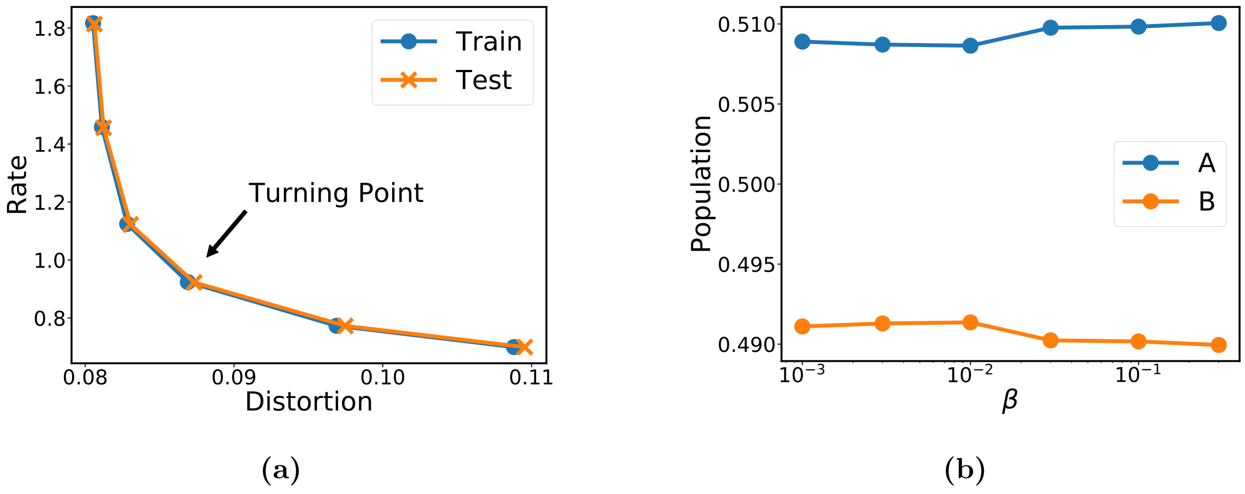


**Supplementary Figure 1:** (a) The Rate-Distortion plot for the double-well analytical potential with the time delay $\Delta t = 2$ *units*. The turning point of the plot ($\beta = 0.03$) is selected to make all the plots in the main text. (b) The robustness of the fractional population to the choice of $\beta$.

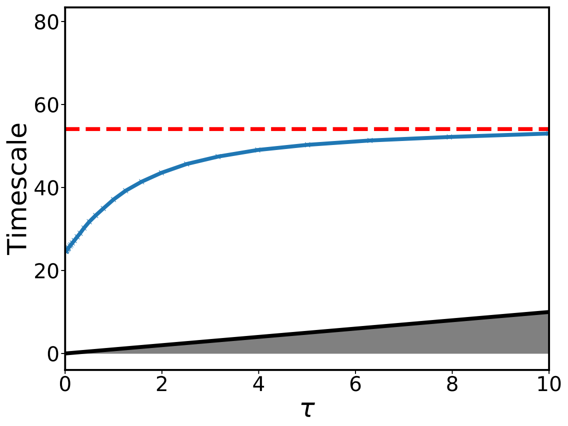


**Supplementary Figure 2:** The implied timescale of the transition between state A and B. $\tau$ represents the lag time used to calculate the transition probability. The blue line represents the implied timescale of the transition between state A and B, the red dotted line corresponds to the converged implied timescale ($t_2 = 54$ *units*), and the grey area represents the timescale that is smaller than the lag time.

## V. FOUR-WELL ANALYTICAL POTENTIAL

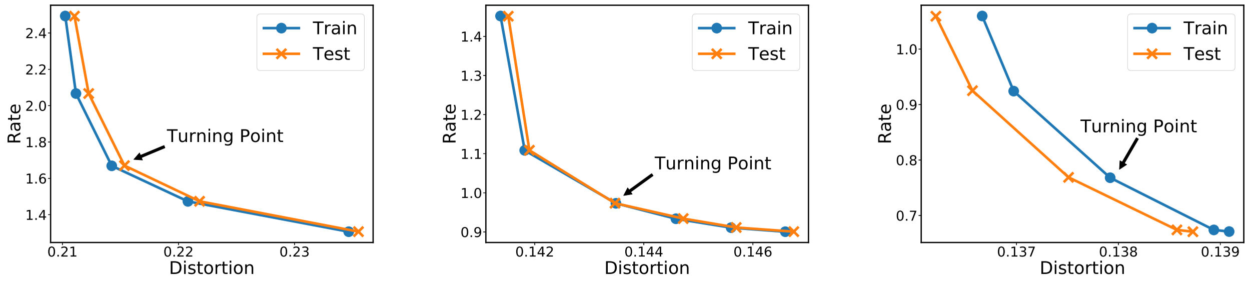


**(a)** $\Delta t = 0.5$ **(b)** $\Delta t = 2$ **(c)** $\Delta t = 10$

**Supplementary Figure 3:** The Rate-Distortion plot for the four-well analytical potential with the time delay $\Delta t = 0.5$ *units* (a), $\Delta t = 2$ *units* (b), $\Delta t = 10$ *units* (c). The turning point of the plot ($\beta = 0.01$) is selected to make all the plots in the main text.

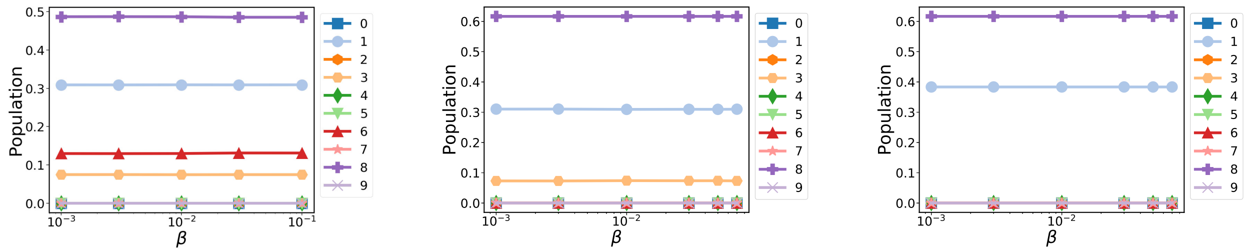


**(a)** $\Delta t = 0.5$ **(b)** $\Delta t = 2$ **(c)** $\Delta t = 10$

**Supplementary Figure 4:** The robustness of the fractional population to the choice of $\beta$ with the time delay $\Delta t = 0.5$ *units* (a), $\Delta t = 2$ *units* (b), $\Delta t = 10$ *units* (c).

## VI. ALANINE DIPEPTIDE IN VACUUM

### A. Discretization of $\phi$

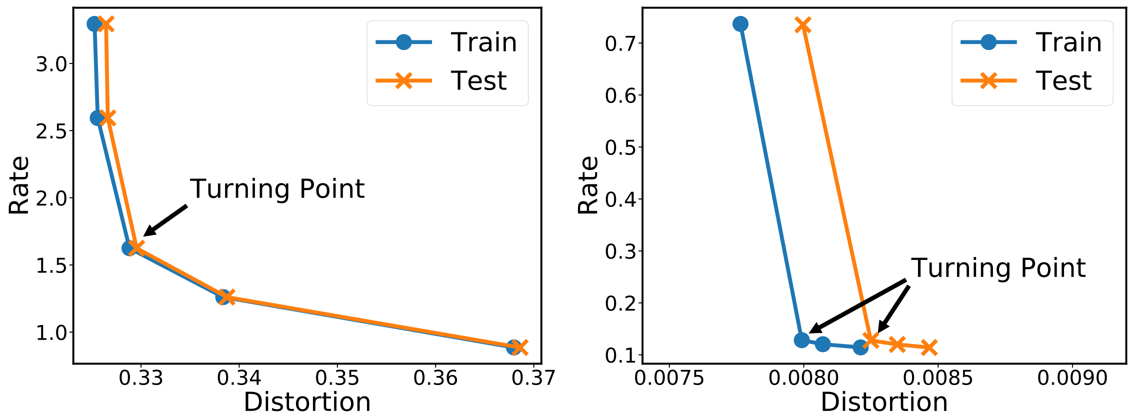


**(a)** $\Delta t = 0.5\ ps$ **(b)** $\Delta t = 2\ ps$

**Supplementary Figure 5:** The Rate-Distortion plot for the alanine dipeptide using the discretization of $\phi$ as the initial guess. Different time delay $\Delta t = 0.5\ ps$ (a), $\Delta t = 2\ ps$ (b) are used to select the turning point $\beta = 0.01$.

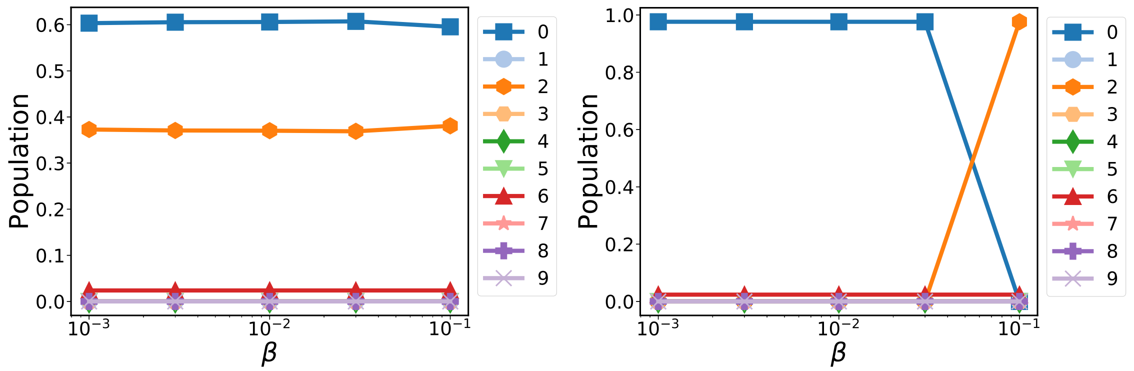


**(a)** $\Delta t = 0.5\ ps$ **(b)** $\Delta t = 2\ ps$

**Supplementary Figure 6:** The robustness of the fractional population to the choice of $\beta$ for the alanine dipeptide using the discretization of $\phi$ as the initial guess. Different time delay $\Delta t = 0.5\ ps$ (a), $\Delta t = 2\ ps$ (b) are shown.

## B. Discretization of $\psi$

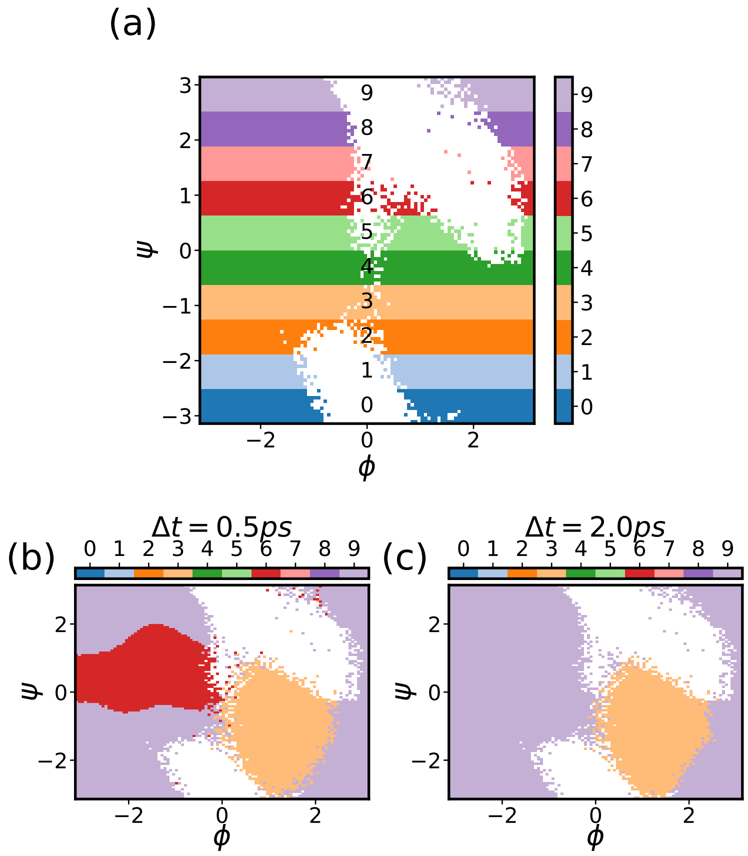


**Supplementary Figure 7:** The time-dependent discrete-state representation of alanine dipeptide in vacuum using the discretization of $\psi$ as the inital state labels. The initial state labels are shown in (a). A three-state representation was learned by using the time delay $\Delta t = 0.5ps$ (b), and a two-state representation was obtained by using the time delay $\Delta t = 2ps$ (c). (b,c) are the state labels projected to $\phi$-$\psi$ space. The color (or state label) in each grids only suggests the proportion of samples belonging to that label is the largest. $\beta = 0.01$ is used to generate (b,c).

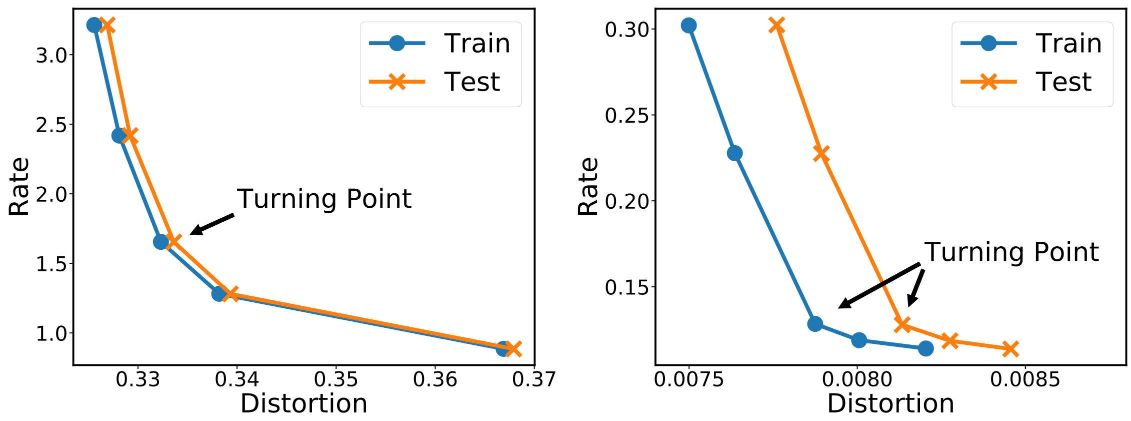


**(a)** $\Delta t = 0.5\ ps$ **(b)** $\Delta t = 2\ ps$

**Supplementary Figure 8:** The Rate-Distortion plot for the alanine dipeptide using the discretization of $\psi$ as the initial guess. Different time delay $\Delta t = 0.5\ units$ (a), $\Delta t = 2\ units$ (b) are used to select the turning point $\beta = 0.01$.

## C. Discretization of $\theta$

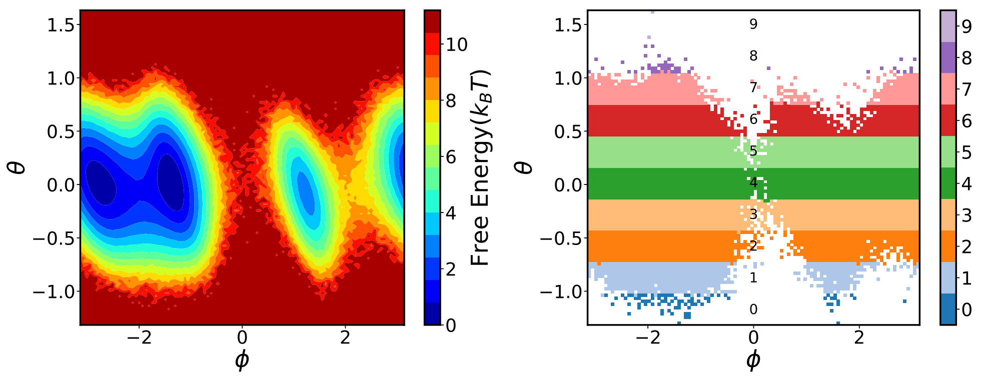


**(a)** **(b)**

**Supplementary Figure 9:** (a) The generated free energy surface for alanine dipeptide in vacuum at 450K along the dihedral angles $\phi$ and $\theta$. (b) The initial state labels generated from the discretization along $\theta$.

## SUPPLEMENTARY REFERENCES


[1]C. E. Shannon, IRE Nat. Conv. Rec **4**, 1 (1959).

[2]A. Alemi, B. Poole, I. Fischer, J. Dillon, R. A. Saurus, and K. Murphy, (2018).

[3]Y. M. Berezansky, Z. G. Sheftel, and G. F. Us, "Spectral decomposition of compact selfadjoint operators. analytic functions of operators," in Functional Analysis (Springer, 1996) pp. 355–384.

[4]F. Noé and F. Nuske, Multiscale Modeling Simulation **11**, 635 (2013).

[5]W. C. Swope, J. W. Pitera, and F. Suits, The Journal of Physical Chemistry B **108**, 6571 (2004).
